# Supplementary material for: Differentially Private Multi-Sampling from Distributions
Source: arXiv:2412.10512 source file (2024-12-13)
Supplement: Supplementary file 1 [file sandbox.tex]

\ifnum\showsandbox=1
\section{Sandbox}
Let $M_\gamma:[L,R]\to [L,R]$ be the local mechanism that, on input $i$, draws a sample from the distribution whose density at $x\in [L,R]$ is $\propto \exp(-\gamma |i-x|)$.

The normalizing term is $\int_i^R \exp(-\gamma(x-i))~dx + \int_L^i \exp(-\gamma(i-x))~dx$. The first summand is
\begin{align*}
&\int_i^R \exp(-\gamma(x-i))~dx\\
={}& \exp(\gamma i)\cdot \int_i^R \exp(-\gamma x)~dx\\
={}& -\frac{1}{\gamma} \cdot \exp(\gamma i)\cdot \int_i^R \exp(-\gamma x)~ (-\gamma dx)\\
={}& -\frac{1}{\gamma} \cdot \exp(\gamma i)\cdot [\exp(-\gamma R) -\exp(-\gamma i)]\\
={}& \frac{1}{\gamma} \cdot [1-\exp(-\gamma (R-i)) ]\\
\end{align*}
Similar steps lead to
$$
\int_{-R}^i \exp(-\gamma(i-x))~dx = \frac{1}{\gamma} \cdot  [1-\exp(-\gamma (i-L)) ]
$$

Input can vary from $L$ to $R$. This means, for any $x$, $\exp(-\gamma|i-x|)$ has a maximum of 1 when $x=i$ and a minimum of $\exp(-\gamma (R-L))$ when $i=L$ and $x=R$ (or vice versa). Meanwhile, the extreme values taken by the normalizing term are $\frac{1}{\gamma} [1-\exp(-\gamma(R-L))]$ and $\frac{1}{\gamma} [2-2\exp(-\gamma(R-L)/2)]$. We use these extrema to calculate privacy loss. Specifically, when $\gamma = \eps_0/2(R-L)$, $\exp(-\gamma|i-x|)$ can change by a factor of $\leq \eps_0/2$ and the normalizing term can change by at most
\begin{align*}
&\ln \paren{\frac{2-2\exp(-\gamma(R-L)/2)}{1-\exp(-\gamma(R-L))} }\\
={}& \ln \paren{ 2 \cdot \frac{1-\exp(-\eps_0/4)}{1-\exp(-\eps_0/2)} }\\
<{}& \eps_0/2
\end{align*}
Thus, $M_\gamma$ ensures $\eps_0$-local DP.

The mass placed on $[i-\Delta, i+\Delta]$---for some $\Delta\leq \min(i-L,R-i)$---is 
\begin{align*}
&\frac{\int_i^{i+\Delta} \exp(-\gamma(x-i))~dx + \int_{i-\Delta}^i \exp(-\gamma(i-x))~dx}{\int_i^R \exp(-\gamma(x-i))~dx + \int_L^i \exp(-\gamma(i-x))~dx}\\
={}& \frac{2-2\exp(-\gamma \Delta)}{[1-\exp(-\gamma (R-i))] + [1-\exp(-\gamma (i-L))]}
\end{align*}
Therefore the mass placed outside of $[i-\Delta, i+\Delta]$ is
\begin{align*}
&1-  \frac{2-2\exp(-\gamma \Delta)}{[1-\exp(-\gamma (R-i))] + [1-\exp(-\gamma (i-L))]}\\
={}& \frac{[\exp(-\gamma \Delta)-\exp(-\gamma (R-i))] + [\exp(-\gamma \Delta)-\exp(-\gamma (i-L))]}{[1-\exp(-\gamma (R-i))] + [1-\exp(-\gamma (i-L))]}\\
\leq{}& \frac{[\exp(-\gamma \Delta)-\exp(-\gamma (R-i))] + [\exp(-\gamma \Delta)-\exp(-\gamma (i-L))]}{\max\paren{[1-\exp(-\gamma (R-i))] , [1-\exp(-\gamma (i-L))]} }\\
\leq{}& 2\cdot \frac{\max \paren{[\exp(-\gamma \Delta)-\exp(-\gamma (R-i))] , [\exp(-\gamma \Delta)-\exp(-\gamma (i-L))]}}{\max\paren{[1-\exp(-\gamma (R-i))] , [1-\exp(-\gamma (i-L))]} }\\
\leq{}& 2\cdot \frac{\exp(-\gamma\Delta) }{1- \exp(-\gamma(R-L))}\\
={}& 2\cdot \frac{\exp(-\eps_0\Delta/2(R-L)) }{1- \exp(-\eps_0/2)}
\end{align*}
We would like to choose $\Delta$ such that the above is bounded by $\beta$

For $\eps<1$, Feldman et al.'s general amplification by shuffling theorem implies that a local privacy loss of $\eps_0 = \ln(\eps^2 n / 64\ln(4/\delta))$ becomes a shuffled privacy loss of $\eps$. Thus, the desired mass bound can be rewritten as
\begin{align*}
2\cdot \frac{\paren{\frac{8\sqrt{\ln(4/\delta)}} {\eps\sqrt{n}}}^{\Delta/(R-L)}}{1- \frac{8\sqrt{\ln(4/\delta)}} {\eps\sqrt{n}} } \leq{}& \beta\\
\paren{\frac{8\sqrt{\ln(4/\delta)}} {\eps\sqrt{n}}}^{\Delta/(R-L)} \leq{}& \frac{\beta}{2} \cdot \paren{ 1- \frac{8\sqrt{\ln(4/\delta)}} {\eps\sqrt{n}}}\\
\Delta \geq{}& (R-L)\cdot \frac{-\ln \paren{ \frac{\beta}{2} \cdot \paren{ 1- \frac{8\sqrt{\ln(4/\delta)}} {\eps\sqrt{n}}} } }{\ln \frac {\eps\sqrt{n}} {8\sqrt{\ln(4/\delta)}}  }
\end{align*}
For sufficiently large $n$,  the quantity $\frac{8\sqrt{\ln(4/\delta)}} {\eps\sqrt{n}}$ is at most $1/10$ so that it suffices for
$$
\Delta \geq (R-L)\cdot \frac{\ln \paren{ \frac{20}{9\beta} }}{\ln \frac{\eps\sqrt{n}} {8\sqrt{\ln(4/\delta)}}  }
$$
\fi
