# Supplementary material for: Differentially Private Multi-Sampling from Distributions
Source: arXiv:2412.10512 source file (2024-12-13)
Supplement: Supplementary file 2 [file product-distributions.tex]

\subsection{DP Weak Multi-sampling for Product Distributions}

Idea: replicate Ghazi et al.'s algorithm \cite{Ghazi00M23}, except we use a unary / fixed-point representation. Specifically, instead of computing a mean $q$ of truncated vectors, we expand each vector into $g$ vectors consisting entirely of zeroes and ones. The average of the values in coordinate $j$ is $q_j$. Note that the $g$ vectors need to be randomized in two different ways: first, there should be no correlation between columns, second, $q_j \cdot g$ may not be an integer so we use randomized rounding.

The clipping operation corresponds to choosing random entries in each column and flipping them.

The sampling operation corresponds to picking a uniformly random row of the table (after clipping).

Idea: to produce multiple samples, we replace one user's $g$ rows with a fresh user's $g$ rows and then apply clipping again.

To reason about the privacy of the single sample version, we need to show that the distribution from running our algorithm and the distribution from Ghazi et. al. are close. (depends on the value $g$ which should be large $\sim \log 1/\delta$
