# Supplementary material for: Differentially Private Multi-Sampling from Distributions
Source: arXiv:2412.10512 source file (2024-12-13)
Supplement: Supplementary file 3 [file deprecated-strong-lower-bound.tex]

\subsection{A Generic Recipe for Strong Multi-Sampling Lower bounds}

Here we develop a generic method of proving lower bounds for strong multi-sampling. We lightly generalize the notion of \emph{sample amplification} by Axelrod et al.

\begin{defn}[Sample Amplification \cite{AGSV19}]
    A family of distributions $\cD$ over some domain $\cX$ admits an $(n,m,\alpha)$-amplification procedure if there is a randomized algorithm $A: \cX^n\to \cX^m$ with the following property: if it is given $n$ i.i.d. samples from any $\bD\in\cD$, the $m$ random variables it outputs has joint distribution $\bJ$ satisfying $\tvd{\bD^{\otimes m}-\bJ}\leq \alpha$.
\end{defn}

It is easy to see that an algorithm that performs strong $(m,\alpha)$-sampling with sample complexity $n$ is a $(n,m,\alpha)$-amplification procedure.

\medskip

Suppose the following two statements are true:
\begin{enumerate}
    \item $\cD$ does not admit an $(n,m,\alpha)$-amplification procedure, so there does not exist an strong $(m, \alpha)$-sampler for $\cD$ with sample complexity $n$.
    \item the sample complexity of $\alpha$-sampling under DP is at least $n'$.
\end{enumerate}

The above implies there cannot be a strong $(m,\alpha)$-sampler for $\cD$ under DP with sample complexity $< n/2 + n'/2$. Suppose there were. We could use it as an amplification procedure but when $n>n'$ this would contradict the lower bound in point 1 (because $n/2 + n'/2 \leq n$). Otherwise, we could simply report the first random variable output of the strong multi-sampler as a single-sampler; doing so would contradict the lower bound in point 2 because $n/2+n'/2 \leq n'$.


\subsection{Lower bound for Strong Multi-Sampling of Finite Distributions}

Axelrod et al. prove the following result about distributions over $[k]$ \cite[Theorem 1]{AGSV19}:

\begin{thm}[Lower bound for amplifying $k$-ary samples]
    There is a constant $c$ such that for every sufficiently large $k$, distributions over $[k]$ do not admit an $(n,n+cn/\sqrt{k},1/3)$-amplification procedure.
\end{thm}
\begin{coro}
    There is a constant $c$ such that for every sufficiently large $k$ and any $\alpha \leq 1/3$, distributions over $[k]$ do not admit an $(n,n+cn/\sqrt{k},\alpha)$-amplification procedure.
\end{coro}
\begin{proof}
    Suppose such an amplification procedure exists. It is also an $(n,n+cn/\sqrt{k},1/3)$-amplification procedure, by virtue of the fact that $\alpha \leq 1/3$ and transitivity of distances. But this contradicts the theorem.
\end{proof}

Meanwhile, Raskhodnikova et al. give a lower bound for approximate DP single-sampling:

\begin{thm}[Lower bound for single-sampling $k$-ary distributions \cite{RSSS21}]
For any $\eps\in(0,1)$, $\delta \in (0, 1/5000n]$, and $\alpha \in (0,1/50]$, any $(\eps,\delta)$-DP $\alpha$-sampler for distributions over $[k]$ must have sample complexity $n = \Omega(k/\alpha\eps)$.
\end{thm}

Combining the two theorems above results in our lower bound:

\begin{thm}[Lower bound for strong multi-sampling $k$-ary distributions]
\label{thm:strong-k-lower-bound}
For any $\eps\in(0,1)$ and $\delta \in (0, 1/5000n]$, any $(\eps,\delta)$-DP strong $(m,\alpha)$-sampler for distributions over sufficiently large $[k]$ must have sample complexity $n \geq m\cdot\paren{1+\frac{c}{\sqrt{k}}}^{-1} + c'\cdot \frac{k}{\alpha\eps}$.
\end{thm}
