# Supplementary material for: Differentially Private Multi-Sampling from Distributions
Source: arXiv:2412.10512 source file (2024-12-13)
Supplement: Supplementary file 4 [file deprecated-upper-bounds.tex]

%We take the following approach: privately identify a $1-\alpha$ confidence interval of the distribution and run \shurr\ assuming that the support is that interval. We show that it is possible to have a sample complexity scaling with $k$ and the width of the identified confidence interval.

%We remark that our algorithm dynamically requests samples from the distribution instead of consuming all it requires at once.

We give pseudocode for the last case.

\begin{algorithm}
\caption{$\shurr^+$}
\label{alg:shurr-plus}

Run the noise-and-threshold algorithm on $X$ \todo{cite Vadhan, Korolova et al., Bun et al.}.

Let $T \subset \Z$ be the set of integers that the above identified as having nonzero frequency in $X$

\If{$T = \emptyset$} {\Return{$\bot$}}

Let $v$ be the integer in $T$ with the largest estimated frequency

\For{$w \in \{16, 32, 64, 128, \dots \}$}{

    Let $Y$ be $\frac{8}{\eps\alpha}\ln \frac{2w}{\alpha}$ new i.i.d. samples from $\bD$
    
    Run AboveThreshold \todo{cite Dwork \& Roth book} on $Y$ with threshold $1-\alpha$ \& queries $f_0, f_1,\dots, f_w$, where $f_\Delta$ is the fraction of $Y$ that lie in $[v-\Delta, v+\Delta]$

    Break out of for-loop if AboveThreshold responded $\top$ at some iteration $h$
}

Let $Z$ be $m + O(\frac{h}{\eps^2}\log\frac{1}{\delta})$ new i.i.d. samples from $\bD$

\Return{$\shurr(Z)$, with support $[v-h,v+h]$}

\end{algorithm}



% New version
\begin{algorithm}
\caption{$\shurr^+$}
\label{alg:shurr-plus}

\textbf{Parameters}: $\eps, \delta > 0, \alpha, \text{diam}(\cD) \leq w$

\KwIn{$n$ iid samples $X_1,\dots X_n$ from a distribution $\bD$ with support size $|S| \leq k$}
\KwOut{$m$ iid samples $\hat{X}_1,\dots, \hat{X}_m$ from a distribution which is $\alpha$ close to $\bD$ }

Run the noise-and-threshold algorithm on the first $O(\frac{k}{\eps} \log \frac{1}{\delta})$ many samples from $X$ \todo{cite Vadhan, Korolova et al., Bun et al.}.

Let $T \subset \Z$ be the set of integers that the above identified as having nonzero frequency in $X$

\If{$T = \emptyset$} {\Return{$\bot$}}

Let $v$ be the integer in $T$ with the largest estimated frequency
    
Run AboveThreshold \todo{cite Dwork \& Roth book} on the next $\frac{8}{\eps\alpha}\ln \frac{2w}{\alpha}$ samples from $X$ with threshold $1-\alpha$ \& queries $f_0, f_1,\dots, f_w$, where $f_\Delta$ is the fraction of $Y$ that lie in $[v-\Delta, v+\Delta]$

Let $f_h$ be the first query where AboveThreshold responded $\top$

Let $Z$ be the remaining $m + O(\frac{h}{\eps^2}\log\frac{1}{\delta})$ samples from $X$

\Return{$\shurr(Z)$}
\end{algorithm}

Differential privacy of $\shurr^+$ follows from applying closure under composition: noise-and-threshold, AboveThreshold, and the original \shurr are each differentially private. It remains to argue that the algorithm performs weak multi-sampling.

To do so, we prove two lemmas. First, we argue that the algorithm is highly unlikely to produce $\bot$.
\begin{lem}
For $n = O(\frac{k}{\eps}\log \frac{1}{\delta} )$ and any $X$ drawn i.i.d. from a distribution with support size $\leq k$, the probability that $\shurr^+(X)=\bot$ is $< 2\delta$. The probability is over the randomness of both $X$ and $\shurr^+$.
\end{lem}
\begin{proof}
$\bot$ will be reported if noise-and-threshold erases all elements of the support that were present in $X$. An element will be dropped if its noised count falls beneath a threshold $t = O(\frac{1}{\eps}\log \frac{1}{\delta} )$. So it suffices to argue that there is some element of the support that has noisy count greater than $t$, except with probability $\leq 2\delta$.

Observe that the mode of $\bD$ has probability mass $\geq 1/k$. By a multiplicative Chernoff bound, our choice of $n$ ensures the mode will have count exceeding $2t$ in $X$, except with probability $\leq \delta$. We also know that adding Laplace noise to $2t$ will result in a value less than $t$ with probability $\leq \delta$. A union bound completes the proof.
\end{proof}

\begin{lem}
    For $n > \frac{2}{\alpha^2}\ln \frac{2}{\beta}$, an interval $I$ of the form $[v-\Delta,v+\Delta]$ containing $> 1-\alpha$ fraction of samples from $\bD$ contains $1-2\alpha$ of the mass except with probability $\beta$.
\end{lem}

\begin{proof}
    Let $\tau = 1-\alpha - \sqrt{\frac{1}{2n}\ln 2/\beta}$. Let $I^*$ be the largest interval of the form $[v-\Delta, v+\Delta]$ such that $I^*$ has $\leq \tau$ mass. By Hoeffding's, the number of elements in $I^*$ is bounded by $n \cdot \tau + \sqrt{\frac{n}{2}\ln 2/\beta} = n\cdot (1-\alpha)$ with probability $\geq 1-\beta$. Conditioned on this event, any interval $I\supset I^*$ that contains $> n\cdot(1-\alpha)$ points must have mass greater than $\tau \geq 1-2\alpha$
\end{proof}
---


\begin{proof}
    Proof of Lemma 10

    There are three events that are crucial for the algorithm

    \begin{itemize}
        \item The algorithm needs at least one sample from the support of the distribution to not output $\bot$. If $n \geq O(\frac{k}{\eps} \log \frac{1}{\delta})$, then algorithm succesfully receovers one elemnt from the support with probability $\geq 1 - 2\delta$.

        \item Let $diam(\bD)$ be the diameter of the support of the distribution $\bD$. In the worst case, the $v$ chosen by the algorithm may be the smallest or the largest element of the support. Thus above threshold would run for at most $diam(\bD)$ many queries. In other words, $h \leq diam(\bD) $. Now, using the analysis of \href{https://arxiv.org/pdf/2111.02598.pdf}{Dong, Yi} with some changes, one can conclude that all but $O(\frac{1}{\eps} \log \frac{\log diam(\bD)}{\beta})$ samples lie inside the interval returned by AboveThreshold. For these samples to be less than $\alpha $ fraction of the dataset, we need 
        $$ \alpha \geq O(\frac{1}{\eps n} \log \frac{\log diam(\bD)}{\beta})$$
        $$ \implies n \geq O(\frac{1}{\alpha \eps} \log \frac{\log diam(\bD)}{\beta})$$

        Idea : Let I be an interval which has $\geq $ 1- $\alpha$ fraction of the dataset. 
    \end{itemize}
\end{proof}


One idea: if variance is known, then there is potential to use Karwa-Vadhan to find the range of the data. Only problem is that it is originally phrased for Gaussians, but still works for subGaussians (note: Ghazi et al do not tackle subGaussians; their first algorithm heavily relies upon closure of Gaussian distribution under addition)
\begin{itemize}
    \item Easiest case: ``3.1. Estimation of range w/ known variance.'' relies on normality \& knowledge of variance
    \item when variance is not known, use Corollary 1.7 of  \href{https://ocw.mit.edu/courses/18-s997-high-dimensional-statistics-spring-2015/a69e2f53bb2eeb9464520f3027fc61e6_MIT18_S997S15_Chapter1.pdf}{MIT book} to bound the gaps between successive i.i.d. subGaussians. [Do we need to have lower and upper bounds on $\sigma$, as the pseudocode apparently does?]
\end{itemize}


Second idea: binary search

The third idea is to use the quantile finding algorithm for infinte discrete domains from \cite{DongY23} to find the $\alpha/2^{th}$ and the $1 - \alpha/2^{th}$ quantiles of the dataset. Next we clip the input samples within the interval formed the two quantiles. Now we can run the subsampled randomized response on the clipped samples with the interval as domain.

\noindent \todo{Need to add notation that $X_{\alpha}$ means $\alpha$ quantile of the dataset and $q_{\alpha}$ means the $\alpha$ quantile for the distribution. Also define rad and diam}

\begin{algorithm}
\caption{$\mathsf{ClipSuRR}$, Clipping + Subsampled Randomized Response }

\textbf{Parameters} : $\eps, \delta > 0, \alpha, \beta$

\KwIn{$n$ samples $X_1,\dots X_n$ from a distribution over $\Z$}
\KwOut{One sample $\hat{X}$ from a distribution over $\Z$}

$\tilde{X}_{\alpha/2} \gets$ $\mathsf{InfinteDomainQuantile}$($X_1, \dots, X_n, \frac{\alpha}{2}, \frac{\eps}{2}, \frac{\beta}{2}$) 

$\tilde{X}_{1 - \alpha/2} \gets$ $\mathsf{InfinteDomainQuantile}$($X_1, \dots, X_n, 1 - \frac{\alpha}{2}, \frac{\eps}{2}, \frac{\beta}{2}$) 

Assign $I \gets [\tilde{X}_{\alpha/2}, \tilde{X}_{1 - \alpha/2}]$

Clip the input samples $X_1, \dots, X_n$ to the interval $I$

Compute $\hat{X}$ by running $\mathsf{SuRR}$ with the clipped samples as input and with $I$ as the domain
\end{algorithm}

\begin{theorem}
    $\mathsf{ClipSuRR}$ is an $(\eps, \delta)$ differentially private algorithm that takes $n$ samples as input from a distribution on $\Z$ and performs $\alpha$ single private sampling with sample complexity $n \geq f(\eps, \alpha, )$
\end{theorem}
\begin{proof}
    To Do
\end{proof}

\begin{theorem}[Theorem 3.5 \cite{DongY23}]
    Given any $\eps, \beta$, any dataset $D$ over $\Z^n$ and for any $\gamma \in (1/n, 1)$ , if 
    $$ n \geq \frac{c_1}{\eps} \log \paren{ \frac{\text{rad}(D)}{\beta}}, $$
    where $c_1$ is a universal constant, then with probability at least $1 - \beta$, the $\eps$ - differentially private algorithm  
    $\mathsf{InfinteDomainQuantile}$ returns a value $\tilde{X}_{\gamma}$ such that

    $$ X_{\gamma - \tau} \leq \tilde{X}_{\gamma} \leq X_{\gamma + \tau}, $$
    where $$\tau = O \paren{ \frac{1}{\eps n} \log \paren{\frac{\text{diam}(D)}{\beta}}}$$
\end{theorem}

\begin{lemma}
    Let $X_1, X_2, \dots, X_n$ be a dataset of $n$ iid samples generated from a distribution $\mathcal{D}$. Let $q_{\gamma}$ denote the population $\gamma$-quantile for $\mathcal{D}$ and $X_{\gamma}$ denote the empirical $\gamma$-quantile computed from the dataset.

    $$\text{For } \Delta \geq \sqrt{\frac{1}{2 n} \log \frac{1}{\beta}}, $$ 
    $$\Pr(X_{\gamma} < q_{\gamma - \Delta}) \leq \beta \text{ and } \Pr(X_{\gamma} > q_{\gamma + \Delta}) \leq \beta$$

\end{lemma}
\begin{proof}
    Follows from a simple application of Hoeffding's inequlity.
\end{proof}

\begin{lemma}
    Given any $\eps, \beta$, any dataset $D$ over $\Z^n$ where each record is generated from a distribution $\mathcal{D}$ over $\Z$ and for any $\gamma \in (1/n, 1)$ , if 
    $$ n \geq \frac{c_1}{\eps} \log \paren{ \frac{\text{rad}(D)}{\beta}}, $$
    where $c_1$ is a universal constant, then with probability at least $1 - \beta$, the $\eps$ - differentially private algorithm  
    $\mathsf{InfinteDomainQuantile}$ returns a value $\tilde{X}_{\gamma}$ such that

    $$ q_{\gamma - \eta} \leq \tilde{X}_{\gamma} \leq q_{\gamma + \eta}, $$
    where $$\eta = O \paren{ \frac{1}{\eps n} \log \paren{\frac{\text{diam}(D)}{\beta}} + \sqrt{ \frac{1}{n} \log \paren{\frac{1}{\beta}}}}$$
\end{lemma}
\begin{proof}
    Fix $\Delta = \sqrt{\frac{1}{2 n} \log \frac{3}{\beta}}$. Let us define three events $\mathcal{E}_1, \mathcal{E}_2$ and $\mathcal{E}_3$. 
    $$ \mathcal{E}_1 : X_{\gamma - \tau} \leq \tilde{X}_{\gamma} \leq X_{\gamma + \tau}$$
    $$ \mathcal{E}_2 : q_{\gamma - \tau - \Delta} \leq X_{\gamma - \tau}$$
    $$\mathcal{E}_3 : X_{\gamma + \tau} \leq q_{\gamma + \tau + \Delta}$$

    If all the three events hold true then, $$q_{\gamma - \eta} \leq \tilde{X}_{\gamma} \leq q_{\gamma + \eta}, \text{ where } \eta = \tau + \Delta$$.

    Using Theorem 10, we know that $\Pr(\overline{\mathcal{E}_1}) \leq \beta/3$. Using Lemma 12 and the value of $\Delta$ fixed above, both $\Pr(\overline{\mathcal{E}_2})$ and $\Pr(\overline{\mathcal{E}_3})$ are $\leq \beta/3$. Taking a union bound over these events and taking the complement, we get that 
    $$\Pr(q_{\gamma - \eta} \leq \tilde{X}_{\gamma} \leq q_{\gamma + \eta}) \geq 1 - \beta$$

    Note that, from Theorem 10 we know that $$\tau = O\paren{ \frac{1}{\eps n} \log \paren{\frac{\text{diam}(D)}{\beta}}}$$ Thus, $$\eta = \tau + \Delta = O\paren{ \frac{1}{\eps n} \log \paren{\frac{\text{diam}(D)}{\beta}} + \sqrt{ \frac{1}{n} \log \paren{\frac{1}{\beta}}}}.$$
\end{proof}
