# Supplementary material for: Differentially Private Multi-Sampling from Distributions
Source: arXiv:2412.10512 source file (2024-12-13)
Supplement: Supplementary file 5 [file old_notes.tex]

\documentclass{article}
\usepackage{graphicx} % Required for inserting images
\usepackage{biblatex}
\addbibresource{refs.bib}
\usepackage{preamble}


\title{DP Multi-Sampling}
\author{Albert Cheu and Debanuj Nayak}
\date{\today}

\begin{document}


\maketitle

\section{Warmup: One DP Sample for Finite Domain}
Given $n$ samples $X_1,\dots X_n$ from a distribution over $[k]$, we pick one $i\in[n]$ uniformly at random and apply $\eps_0$ randomized response: place $\propto \exp(\eps_0)$ weight on $X_i$ and place $\propto 1$ weight on all other elements in $[k]$.

For any outcome $y\in [k]$ and $X,X'$ that differ on index $j$,
\begin{align*}
    &\frac{\pr{}{M(X)=y}}{\pr{}{M(X')=y}}\\
    ={}& \frac{\sum_i \frac{1}{n} \pr{}{RR(X_i)=y} }{\sum_i \frac{1}{n} \pr{}{RR(X'_i)=y}}\\
    ={}& \frac{\sum_{i\neq j} \frac{1}{n} \pr{}{RR(X_i)=y} }{\sum_i \frac{1}{n} \pr{}{RR(X'_i)=y}} + \frac{\frac{1}{n} \pr{}{RR(X_j)=y} }{\sum_i \frac{1}{n} \pr{}{RR(X'_i)=y}}\\
    <{}& \frac{\sum_{i\neq j} \frac{1}{n} \pr{}{RR(X_i)=y} }{\sum_{i\neq j} \frac{1}{n} \pr{}{RR(X'_i)=y}} + \frac{\frac{1}{n} \pr{}{RR(X_j)=y} }{\sum_i \frac{1}{n} \pr{}{RR(X'_i)=y}} \tag{Shrink the denominator}\\
    ={}& 1+\frac{\frac{1}{n} \pr{}{RR(X_j)=y} }{\sum_i \frac{1}{n} \pr{}{RR(X'_i)=y}} \tag{Defn. of $X,X'$}\\
    \leq{}& 1+\frac{\frac{1}{n} \pr{}{RR(X_j)=y} }{\min_i \pr{}{RR(X'_i)=y}} \tag{Mean $\geq$ min}\\
    \leq{}& 1+\frac{1}{n}\exp(\eps_0) \tag{Local DP}
\end{align*}

We will set $\eps_0\gets \ln(\eps \cdot n)$ so that we get $\eps$-dp overall.

What is the deviation from the underlying distribution? Randomized response on any $x\sim \bD$ is equivalent to the mixture $\bD\cdot \frac{\exp(\eps_0)-1}{k-1+\exp(\eps_0)} + \bU \cdot \frac{k}{k-1+\exp(\eps_0)}$ where $\bU$ is the uniform distribution over $[k]$. If we can show the weight $\frac{k}{k-1+\exp(\eps_0)}$ is small, then the TV distance between the mixture and $\bD$ is small.

For $n\geq (k/\alpha+1)/\eps$
\begin{align*}
    &\frac{k}{k-1+\exp(\eps_0)}\\
={}&\frac{k}{k-1+\eps n} \tag{Choice of $\eps_0$}\\
\leq{}&\alpha
\end{align*}

\section{Multiple DP Samples for Finite Domain}

There are two forms of the objective which I call ``weak'' and ``strong.''

\subsection{Weak Multi-Sampling}

In weak multi-sampling, the objective is to use $n$ samples from $\bD$ to produce $m$ i.i.d. samples from a distribution $\bD'$ that is $\alpha$ close to $\bD$ in TV distance. A naive solution would be to execute the randomized-response-with-sampling algorithm on $m$ disjoint datasets. Thus, $n= m \cdot (k /\alpha +1) / \eps$ samples would suffice.

Now I describe a less naive solution: shuffle the inputs uniformly at random and apply $\eps_0$ randomized response to each of the inputs. Instead of using amplification by sampling, we use amplification by shuffling: a result by \href{https://arxiv.org/abs/2012.12803}{ Feldman, McMillan, \& Talwar } implies that there is a universal constant $c$ such that  $(\eps,\delta)$-DP is achieved by setting $\eps_0\gets \ln \left( \frac{  c \eps^2 n }{ \ln (4/\delta) } - 1 \right)$ and shuffling the outcomes of randomized response with parameter $\eps_0$.

To be precise, their bound on the privacy parameter is
\begin{align*}
    &\log \left( 1 + 8(\exp(\eps_0)+1) \left( \sqrt{\frac{k+1}{k}\cdot \frac{\log 4/\delta}{n} \cdot \frac{1}{\exp(\eps_0)+k-1} } + \frac{k+1}{k n} \right) \right)\\
\leq{}& \log \left( 1 + 8(\exp(\eps_0)+1) \left( \sqrt{\frac{3}{2}\cdot \frac{\log 4/\delta}{n} \cdot \frac{1}{\exp(\eps_0)+1} } + \frac{3}{2 n} \right) \right) \tag{$k\geq 2$}\\
\leq{}& \log \left( 1 + 8\cdot \frac{  c \eps^2 n }{ \ln (4/\delta) } \left( \sqrt{\frac{3}{2}\cdot \frac{\log 4/\delta}{n} \cdot \frac{ \ln (4/\delta) }{  c \eps^2 n } } + \frac{3}{2 n} \right) \right)  \tag{Choice of $\eps_0$}\\
={}& \log \left( 1 + 8\eps \cdot \sqrt{3c/2} + \frac{  12c \eps^2  }{ \ln (4/\delta) } \right) \\
<{}& 8\eps \cdot \sqrt{3c/2} + \frac{  12c \eps^2  }{ \ln (4/\delta) } \\
\leq{}& 8\eps \cdot \sqrt{3c/2} + 3c\eps^2 \tag{for $\delta < 4e^{-4}$ }
\end{align*}
For $c=2/(3 \cdot 81)$ and $\eps<4$, this is bounded by $(8/9)\eps + (2/81)\eps^2 < \eps$.

Just as before, the TV distance between $\bD$ and $RR(\bD)$ is $k/(k-1+\exp(\eps_0)$. With the new $\eps_0$ value, it now suffices for $n\geq (k/\alpha +2) \ln(4/\delta)/ c\eps^2$ to bound the distance by $\alpha$.

The upshot is that $O(m + \frac{k}{\alpha \eps^2}  \log\frac{1}{\delta})$ samples suffice for DP weak sampling. $m$ outputs ``come for free'' when the private samples $n$ exceeds a threshold.

\subsection{Strong Multi-Sampling}
In strong multi-sampling, the objective is to use $n$ samples from $\bD$ to produce $m$ random variables whose \emph{joint distribution} is within $\alpha$ of the product distribution $\bD^{\otimes m}$ in TV distance.

A naive solution would be to use the same algorithm as above (shuffled randomized response) but targeting an error tolerance of $\alpha/m$. A union bound ensures the overall TV distance is $\alpha$. Thus, $O(\frac{mk}{\alpha \eps^2}  \log\frac{1}{\delta})$ samples suffice.

Open Question: can we improve this?

\begin{comment}
\subsection{One DP Sample for Continuous-but-Bounded Domain}
Let $\bD$ be a distribution over $[-1,1]$. In this new context, we could replace randomized response with the laplace mechanism.

Suppose $\bD$ places 0.9 mass on $[0.9,1]$. There is at least a $0.9 \cdot (1-\rho_{0.9})$ probability that $\bD*\mathrm{Lap}_b$ lands outside $[-1,1]$, where $\rho_{0.9}$ is the CDF of the laplace distribution at 0.9.
\begin{align*}
    \rho_{0.9} &= \frac{1}{2}+\frac{1}{2}(1-\exp(-0.9/b))\\
    &= 1-\frac{1}{2}\exp(-0.9/b)\\
    0.9 \cdot (1-\rho_{0.9}) &= 0.9\cdot \frac{1}{2}\exp(-0.9/b)\\
\end{align*}
\end{comment}
\section{Lower Bound Strategies for Weak Multi-Sampling}

Debanuj's idea: to learn arbitrary d-dim gaussian under pure dp, we know we need $> d$ public samples. so no pure dp sampling alg can produce values from unbounded domain with finitely many private samples. 

---


Open questions:
\begin{itemize}
\item is the finite domain alg. optimal in the sense that m/n cannot be improved for all m?
\item can we come up with an approx DP Gaussian sampler that is not just repeating Ghazi et al.'s algorithm m times?
\item can we match the lower bound for pure DP Gaussian sampling?
\end{itemize}
%In the case where $\bD$ is a Gaussian, there are $m=d+1$ public samples, and there are $n=\tilde{O}(d^2 (1/\alpha^2 + 1/\alpha\eps))$ private samples, distribution estimation can be done under pure DP. But this means $n$ samples would suffice to estimate a Gaussian under pure DP, which is not possible: there needs to be a dependence on the mean and condition number.

\section{Ideas}
We currently have:
\begin{itemize}
\item single sampler for arbitrary distributions over finite domain
\item weak multi-sampler for arbitrary distributions over finite domain
\end{itemize}

\begin{table}[]
    \centering
    \begin{tabular}{|c|c|c|c|} \hline
        \multirow{2}{*}{Domain} & \multirow{2}{*}{Distribution} & \multicolumn{2}{c|}{Sample complexity to produce\dots} \\ \cline{3-4}
        & & 1 Sample & $m$ Samples \\ \hline
        $k$ & arbitrary & $k/\alpha \eps$ & $m + \frac{k}{\alpha\eps^2}\log \frac{1}{\delta}$ \\ \hline
        $k$ & $1-\alpha$ mass placed in window of size $w$ & $(\log k + w)/\alpha \eps$ via binary search& \\ \hline
        $k$ & $\sigma$ known & $\tilde{O}(\sigma/\alpha\eps)$ via noise-and-drop & \\ \hline
        $\Z$ & $\sigma$ known & $\tilde{O}(\sigma/\alpha\eps)$ & \\ \hline
        $\Z$ & $\Pois(\lambda)$ & & \\ \hline
    \end{tabular}
    \caption{Caption}
    \label{tab:my_label}
\end{table}

What don't we have? single- and multi- samplers for 
\begin{itemize}
\item subgaussian or subexponential distributions
\item binomial distributions
\item Poisson distributions
\item product distributions
\item subgaussian or subexponential distributions over reals
\begin{itemize}
\item Ghazi et al. have a mechanism tailored for Gaussian distribution; what about other distributions?
\end{itemize}
\end{itemize}

Proposed algorithm for single-sampling subgaussians or subexponentials with \emph{known stdev} $\sigma$:
\begin{enumerate}
    \item divide dataset in two
    \item Use the first half to find an interval such that the probability mass placed by the distribution on it is $\approx 1-\alpha$
    \begin{enumerate}
        \item Pure DP (finite domain): Binary search the domain until you find the $\approx \alpha/2$ quantile. Then, Binary search for the $\approx 1-\alpha/2$ quantile. Sample complexity is $O(\log(k) (1/\alpha^2 + 1/\alpha\eps)$
        \item Approx DP: noise-and-drop histogram alg. We accumulate error in the nonzero bins, of there are $O(\sigma polylog(1/\alpha))$ for concentrated distributions with stdev $\sigma$. problematic when $\sigma$ is large and unknown
    \end{enumerate}
    \item clamp second half using the two points. We lose $<\alpha$ mass from the distribution
    \item run the subsampled randomized response algorithm on second half
\end{enumerate}

\emph{unknown stdev}: ???

Proposed algorithm for product distributions over $\zo$:
\begin{enumerate}
\item Divide $\alpha,\eps$ over $[d]$
\item Create $d$ datasets of $\zo$ values by dividing each person's string
\item Run our single- or multi- sampler for domain $\zo$ and the divided budget
\end{enumerate}
Single-sampler has sample complexity $\approx d^2/\alpha \eps$, while weak multi-sampler has complexity $\approx m + d^3/\alpha \eps^2$. Naive extension of existing literature consumes $\approx m\cdot d/\alpha \eps$.

\section{Sampling from a Poisson Distribution}

We are given $n$ samples, $X_1, X_2, \dots X_n$ from an unknown Poisson distribution i.e. $Poi(\lambda)$ where $\lambda$ is unknown.

\textbf{Proposed Algorithm}
\begin{enumerate}
\item Divide the dataset into two parts.
    \item Run a DP quantile finding algorithm on the first dataset to find the $\alpha/2$th and the $1 - \alpha/2$th quantiles. (Need to check - How?)

    \item Run stable histogram with exponenetially increasing bins. ( we have an interval whose length is bounded)

    \item I can run binary search (option1 : Just do binary search with laplace noise option2 : threshold queries inside the interval.

    
    \item Clamp all the points in the second dataset within the range given by the two quantiles.
    \item Run the DP sampling algorithm for arbitrary distributions over a finite domain over these clamped datapoints.
\end{enumerate}

\begin{lemma}
    Let $X_1, X_2, \dots, X_n$ be a dataset of $n$ iid samples generated from a distribution $\mathcal{D}$. Let $q_{\gamma}$ denote the population $\gamma$-quantile for $\mathcal{D}$ and $\hat{q}_{\gamma}$ denote the empirical $\gamma$-quantile computed from a dataset. 

    $$\text{If } n \geq \frac{2}{\gamma^2} \log \frac{2}{\beta}, \text{ then, }\Pr(q_{\gamma/2} \leq \hat{q}_{\gamma} \leq q_{3\gamma/2}) \geq 1 - \beta,$$

    $$\text{If } n \geq \frac{1}{2 \gamma^2} \log \frac{1}{\beta}, \text{ then, }\Pr(\hat{q}_{\gamma} > q_{2\gamma}) \leq \beta,$$

    $$\text{If } n \geq \frac{1}{2 (F(q_{\alpha} + t) - \alpha)^2} \log \frac{1}{\beta}, \text{ then, }\Pr(\hat{q}_{\alpha} > q_{\alpha} + t) \leq \beta,$$

    $$\text{If } n \geq \frac{1}{2 (\alpha - F(q_{\alpha} - t))^2} \log \frac{1}{\beta}, \text{ then, }\Pr(\hat{q}_{\alpha} < q_{\alpha} - t) \leq \beta,$$

    $$\text{If } n \geq \frac{1}{2 \Delta^2} \log \frac{1}{\beta}, \text{ then, }\Pr(\hat{q}_{\alpha} > q_{\alpha + \Delta}) \leq \beta,$$

    $$\text{If } n \geq \frac{1}{2 \Delta^2} \log \frac{1}{\beta}, \text{ then, }\Pr(\hat{q}_{\alpha} < q_{\alpha - \Delta}) \leq \beta.$$
\end{lemma}
\begin{proof}
    Let $Y_1, Y_2$ denote the no. of data points in the dataset which are less than $q_{\gamma/2} $ and greater than $q_{3\gamma/2}$ respectively. By the definition of the population quantile, we know that $\E{Y_1} = \frac{\gamma n}{2}$ and $\E{Y_2} = \frac{3\gamma n}{2}$. Let $\mathcal{E}_1$ and $\mathcal{E}_2$ denote the events $Y_1 > \gamma n$ and $Y_2 < \gamma n$. Note that $\mathcal{E}_1$ can be interpreted as the event $\hat{q}_{\gamma} < q_{\gamma/2}$ as the initial $\gamma $ fraction of the $n$ samples already lies before $q_{\gamma/2}$. Similarly, one can conclude that the event $\mathcal{E}_2$ is equal to $\hat{q}_{\gamma} > q_{3\gamma/2}$ as less than $\gamma $ fraction of the $n$ samples lie till $q_{3\gamma/2}$.
    

    $$\Pr(\mathcal{E}_1) = \Pr(Y_1 > \gamma n) = \Pr(Y_1 - \E{Y_1} > \frac{\gamma n}{2}) \leq \exp \left(\frac{- 2 \gamma^2 n^2}{4 n} \right) = \exp \left(\frac{- \gamma^2 n}{2} \right) \leq  \frac{\beta}{2}$$

    $$\Pr(\mathcal{E}_2) = \Pr(Y_2 < \gamma n) = \Pr(\E{Y_2} - Y_2 > \frac{\gamma n}{2}) \leq \exp \left(\frac{- 2 \gamma^2 n^2}{4 n} \right) = \exp \left(\frac{- \gamma^2 n}{2} \right) \leq  \frac{\beta}{2} $$

    \noindent The inequalities mentioned hold true using Hoeffding's concentration inequality. Using union bound,  $\Pr(\mathcal{E}_1 \cup \mathcal{E}_1) \leq \beta$ which implies that $\Pr(\neg \mathcal{E}_1 \cap \neg \mathcal{E}_2) \geq 1 - \beta.$ This concludes the proof.
\end{proof}

\subsection{DP quantile estimation algorithm for unbounded data universe}

All of the existing work on algorithms for estimating quantiles privately from a dataset require that the data universe be bounded. However, in our problem, we are working with samples from a Poisson distribution and thus the data universe is the set of natural numbers which is unbounded. Thus we need to develop new methods to estimate quantiles here.

\subsubsection{Stability based histograms with exponentially increasing bin sizes}

Define a sequence of exponentially increasing disjoint bins $\{ B_j\}_{j \in \N}$ such that $B_j$ is the set of all natural numbers in the interval $\{2^j - 1, \dots , 2(2^j - 1)\}$. In particular $B_0 = \{0\}, B_1 = \{1,2\}, B_2 = \{3,4,5,6\}$ and so on.

\noindent Also define the set of counting queries $Q^{\text{Bin}}(\N)$ as the set $\{f_j\}_{j \in \N}$ where $f_j$ denotes the fraction of data points in the dataset that lie inside bin $B_j$. We can now adapt the stability based histogam approach of Bun et al. \cite{BunNS19} to answer all the queries in $Q^{\text{Bin}}(\N)$.

\begin{lemma}
    For all $n \in \N, \eps \in (0, \ln n)$ and $\delta \in (0, 1/n)$ there is an $(\eps, \delta)$ differentially private algorithms that on every dataset $D \in \N^n$ can answer with high probability all of the counting queries in $Q^{\text{Bin}}(\N)$ to within error
    $$O\left(\frac{\log 1/\delta}{\eps n} \right)$$
\end{lemma}


\noindent Define $a_j$ as the differentially private response to the query $f_j$. Thus $|a_j - f_j| \leq O\left(\frac{\log 1/\delta}{\eps n} \right)$ for all $j \in \N$.

\noindent Define $F_k = \sum_{j=0}^k f_j$ and $A_k = \sum_{j=0}^k a_j$. Note that $F_k$ is the fraction of datapoints that lie inside bins $0$ through $k$. 
$$|A_k - F_k| \leq O\left(\frac{k \log 1/\delta}{\eps n} \right)$$

\noindent Let $\ell_\gamma$ be the index of the bin such that $A_{\ell_\gamma - 1} < \gamma$ and $A_{\ell_\gamma} \geq \gamma.$

We need : There should be a lemma that says that with high probability $\hat{q}_\gamma$ lies in Bin $\ell_\gamma$ or a bigger interval.

what we have is 



\section{Weak Multi-Sampling from Gaussian Distributions}

\subsection{One-Dimensional Case}

\noindent  Consider the class of one dimensional Gaussian distributions with arbitrary known variance $\sigma^2$. Private sampling from this distribution can be reduced to the problem of private sampling from one dimensional distributions with unit variance (variance = 1) using the transform \[ X_{\text{new}} = \frac{x_{\text{old}}}{\sigma}\].

\subsubsection{Building Block: Continuous randomized response}



\noindent Define a probability distribution over any bounded interval $I \subset \mathbb{R}$ of length $R$ such that $a \in I$ using the the following pdf denoted by $f[p,R,a,s](x)$ where
\[f[p,R,a,s](x) = \frac{p}{R} + (1-p)\cdot \mathcal{N}_T(a, s) (x)\]

\noindent where $\mathcal{N}_T(a, s) (x)$ is the pdf of the Gaussian distribution with mean $a$ and variance $s^2$ conditioned to be in the interval $I$. Notice that the distribution as described above is a valid distribution over $I$ since,

\begin{align*}
    \int_{I} f[p,R,a,s](x) dx & = \int_{I} \left[ \frac{p}{R} + (1-p)\cdot \mathcal{N}_T(a, s) (x)\right] dx \\
    & = p\int_{I} \frac{1}{R} dx + (1-p)\int_{I} \mathcal{N}_T(a, s) (x) dx \\
    & = p\cdot\frac{R}{R} + (1-p)\cdot 1 \\
    & = p + (1-p) = 1. \\
\end{align*}



\noindent \textbf{Algorithm : Subsampled Continuous Randomized Response } \\
Input : datapoint $X_1, X_2, \dots X_n$ and an interval  $I = (X_{\text{min}}, X_{\text{max}})$ such that each $X_i \in I$.

\begin{enumerate}
    \item Extend $I$ on both sides by $O(s \sqrt{\log \frac{1}{\alpha}})$. Call this extended interval $I'$.
    \item $R = |I'| = |X_{\text{max}} - X_{\text{min}}|$
    \item Pick $i \in [n]$ uniformly at random.
    \item Sample $z$ from the distribution whose PDF is $f[p,R,X_i,s]$.
    \item Output $z$.
\end{enumerate}

\newpage
\noindent \textbf{Privacy of Subsampled Continuous Randomized Response }\\
Let $X$ and $X'$ are neighbouring datasets that differ at the $j^{th}$ coordinate.
TODO: change to density function.
\begin{align*}
\frac{\Pr{[A(X) \in Y]}}{\Pr{[A(X') \in Y]}} & = \frac{\sum_{i \in [n]} \frac{1}{n}\Pr{[B(X_i) \in Y]}}{\sum_{i \in [n]}\frac{1}{n}\Pr{[B(X'_i) \in Y]}} \\
&< 1+ \frac{\frac{1}{n} \Pr{[B(X_j) \in Y]}}{\sum_{i \in [n]}\frac{1}{n}\Pr{[B(X'_i) \in Y]}} \\
& \leq 1+ \frac{\frac{1}{n} \Pr{[B(X_j) \in Y]}}{\min_{i \in [n]}\Pr{[B(X'_i) \in Y]}} \\
& \leq  1 + \frac{1}{n}\cdot \frac{ \left[\frac{p}{R} + \frac{(1-p)}{\sqrt{2 \pi s^2} }\right]}{\frac{p}{R}} & (\text{Property of } f[p,R,a,s])\\
& \leq 1 + \frac{1}{n}\left[ 1 + \frac{1-p}{p}\cdot \frac{R}{s \sqrt{2 \pi}}\right] \\
& \leq 1 + \frac{1}{n} \exp \left(\frac{1-p}{p}\cdot \frac{R}{s \sqrt{2 \pi}} \right) \\
& \leq 1 + \frac{1}{n}\exp (\varepsilon_0).
\end{align*}
The last inequality will hold for $p\geq R/\eps_0 s \sqrt{2\pi}$ \anote{I simplified the bound (yours remains as a comment)}
%\noindent where the last step follows by setting $p$ as given below, 
%\[p \geq \frac{1}{1 + \frac{\varepsilon_0 s \sqrt{2 \pi}}{R} }.\]

As before we set $\eps_0 = \ln (\eps n)$

\subsubsection{DP Sampling via Continuous randomized response}

\noindent 
\textbf{Algorithm : Single Private Sample from Gaussian with Unit Variance} \\
Input : $X_1, X_2, \dots X_n \sim \mathcal{N}(\mu, 1)$
\begin{enumerate}
    \item Divide the real line into partitions of half-width $h$
    \item Run the open-domain DP histogram algorithm on $(X_1, X_2, \dots X_n )$
    \item $I = (X_{\text{min}}, X_{\text{max}}) \leftarrow $ the interval made by the union of partitions that the DP histogram indicates has data
    \item $X'_1, X'_2, \dots X'_n \leftarrow \text{Clip}(X_1, X_2, \dots X_n, I)$
    \item $z \leftarrow \text{Subsampled Continuous Randomized Response}(X'_1, X'_2, \dots X'_n, I)$
    \item Output $z$.
\end{enumerate}

\begin{conj}
   For every $n \in \N, \eps, \delta, \alpha \in (\frac{1}{100}, 1)$ the above algorithm is a $(\eps, \delta)$ differentially private algorithm which when supplied with $n$ samples from $\cN(\mu, 1)$ and given $\eps, \delta, \alpha$ as input produces a single sample from a distribution $\cD$ where $\tvd{\cN(\mu, 1) - \cD} \leq \alpha$ if 
   \[n \geq \dots f(\eps, \delta, \alpha)\]
\end{conj}
\begin{proof}
    \textbf{Proof of Privacy} : Steps 1 to 3 in the above algorithm can be implemented using algorithm (cite algorithm) which is a $(\eps, \delta)$ differentially private algorithm .  After the clipping operation in step 4, all the new datapoints $X_i'$ for $i \in [n]$ are guaranteed to lie inside $I$. Subsampled continuous randomized response is a $(\eps,0)$ algorithm as shown before. Split the privacy budget such that the first algorithm(cite algorithm) is run with $\eps_1 = \eps/2$ and $\delta_1 = \delta$ and Subsampled continuous randomized response is run with $\eps_2 = \eps/2$. Thus by composition and postprocessing, our algorithm is $(\eps, \delta)$ differentially private.

    \textbf{Proof of Accuracy}: 

     %     \textbf{High-level Proof steps}
    % \begin{itemize}
    % \item After using Karwa-Vadhan (KV), our algorithm clamps data to I and then applies our RR to randomly chosen datum $x$. Our RR is uniform over $I'$ (I extended by some $\ell=O(s \cdot \sqrt{\log(4/\alpha)}$ left and right) with probability p and otherwise is a Gaussian with variance $s^2$ and mean $x$ conditioned on falling in $I'$
    
    % \item Condition on the event that all points lie inside $I$. this fails to occur w.p. $\alpha/4$ if we parameterized the KV alg correctly. [Conditioning on $X_i$'s must lie isnside $I$. Calling this Cond 1].
    
    % \item while still conditioning on that event above, switch to algorithm that does not force the noisy version of the datum to lie inside $I'$. (Here noisy version is w.p. $p$ choose unniformly random from $I'$ else add Gaussian noise to $x$. This costs us only $\alpha/4$ in TV distance. [Cond 1 + Algo change 1]

    % \item Remove the 

    % \item argue that adding Gaussian noise of variance $s^2$ to a Gaussian r.v. does not distort the r.v.'s distribution by more than $\alpha/4$.
    
    % \item argue that the $p< \alpha/4$.
    % \end{itemize} 

    Let $\cD_0$ be the distribution of $z$, the output of our algorithm. Our goal is to bound $\tvd{\cD_0 - \cN(\mu, 1)}$. In order to bound $\tvd{\cD_0 - \cN(\mu, 1)}$, we will describe small changes to the distribution $\cD_0$, step by step until we reach $\cN(\mu, 1)$. Let us describe a series of algorithms denoted by $A_i$ for $i \in \{0 \dots 3\}$,
    \begin{itemize}
        \item $A_0$ represents our algorithm as mentioned above.
        \item $A_1$ is the same as $A_0$ except that in the subsampled continuous randomized response subroutine, we return a sample from a Gaussian $\cN(X_i, s)$ instead of a truncated Gaussian $\cN_T(X_i, s)$ conditioned to be within the interval $I'$ where $X_i$ is the randomly chosen input datapoint.
        \item $A_2$ is the same as $A_1$ except that we always a return a sample from the Gaussian  $\cN(X_i, s)$ not just with probability $1-p$. In other words, a uniform value from $I'$ is never returned.
        \item $A_3$ is the same as $A_2$ except that the clipping in step 4 is not performed.
    \end{itemize}
    Let the corresponding distribution of the output be denoted by $\cD_i$, i.e. the distribution of the output of algorithm $A_i$ is $\cD_i$. Let $\cD_i$ be any distribution and $E$ be some event, we represent the distribution $\cD$ conditioned on the event $E$ as $\cD|_{E}$. Also let $E$ denote the event that all the datapoints lie inside the interval $I$.
    
    Now we can bound $\tvd{\cD_0 - \cN(\mu, 1)}$ as follows

    \begin{align*}
        \dist{\cD_0 - \cN(\mu, 1)} &\leq \dist{\cD_0 - \cD_0|_{E}} + \dist{\cD_0|_{E} - \cD_1|_{E}} + 
        \dist{\cD_1|_{E} - \cD_2|_{E}} +
        \dist{\cD_2|_{E} - \cD_3|_{E}} +
        \dist{\cD_3|_{E} - \cD_3} + \dist{\cD_3 - \cN(\mu, 1)} \\
    \end{align*}

    As mentioned in the Karwa Vadhan paper \cite{KarwaV18} (https://arxiv.org/pdf/1711.03908.pdf), their algorithm can be supplied with an error probability $\beta$ such that all the input datapoints lie within the interval $I$ with probability $\geq 1 - \beta $ and $I$ has a length $\leq O(\sqrt{\log \frac{n}{\beta}})$.

    From above, we know that the event $E$ happens with probability $\geq 1 - \beta $. Using claim 4 from \cite{RaskhodnikovaS06}, we know that $\dist{\cD_0 - \cD_0|_{E}} \leq \frac{\beta}{1 - \beta}$. Similarly, $\dist{\cD_3|_{E} - \cD_3} \leq \frac{\beta}{1 - \beta}$.
    
    Now, to bound $\dist{\cD_0|_{E} - \cD_1|_{E}}$. Note that all the input points $X_i$ for all $i \in [n]$ lie inside the interval $I$.  Thus the total variation distance $\dist{\cD_0|_{E} - \cD_1|_{E}} = (1-p)\dist{\cN_T(X_i, s)|_{E} - \cN(X_i, s)|_{E}}$. 

    
    
    

    

Notice that $\tvd{\cD - \cD|_{E}} \leq \Pr(\overline{E})$. To bound $\tvd{\cD|_{E} - \cD'|_{E}}$ notice that $\cD|_{E}$ is very similar to $\cD'|_{E}$ except that first one involves truncated Gaussian noise and the second one involves Gaussian noise.
\end{proof}
     

Claim: For $\alpha > \dots$ and $s \gets \frac{8}{\eps_0 \sqrt{2\pi}}(1/\alpha)$, the algorithm satisfies $\eps$-DP and the output has TV distance $2\alpha$ from the original distribution.

\begin{proof}
Privacy comes from the previous section + DP histogram algorithm.

\emph{Three sources of error}: Data loss due to DP histogram algorithm, distance caused by Gaussian, and distance caused by randomized response $p$.

If a window has half-width 2, then 95\% of my data will be inside the window. If we break the real line into buckets of half-width 2, then there are one or two buckets that contain 95\% of my data. R is going to be $\leq 2 \cdot (2 \cdot 2) = 8$

$z$ is uniform with prob $p$ and is $N(\mu, s^2 + 1)$ with prob $(1-p)$.

To bound Distance caused by Gaussian, we'll cite this paper: https://arxiv.org/pdf/1810.08693.pdf

If $s \gets \frac{8}{\eps_0 \sqrt{2\pi}}(1/\alpha)$, then
$$\frac{R}{\eps_0 \sqrt{2 \pi}} \cdot \frac{1}{s} = \frac{R}{\eps_0 \sqrt{2 \pi}} \cdot \frac{\eps_0 \sqrt{2\pi} }{8}\cdot \alpha \leq  \alpha$$

\end{proof}

% $ z = z_1 + z_2$ where $z_1$ is $N(\mu, 1)$. $z_2$ is $N(0, s^2 )$. 



\subsection{Multi-Dimensional Case}

Refer to https://arxiv.org/pdf/2306.12549.pdf: Ghazi et al. achieve sample complexity $\approx \sqrt{d}/{\eps}$.


\subsection{Questions}
Is there a private sample for Gaussians under known/bounded varianve under pure DP (possibly using some spherical version of laplace)


% \printbibliography[heading=bibintoc]

\end{document}
